# Supplementary material for: Learning Opinion Summarizers by Selecting Informative Reviews
Source: arXiv:2109.04325 source file (2021-09-09)
Supplement: Supplementary file 2 [file sum_stats_w_meta.tex]

\subsection{Product Meta Fields}
\label{app:summ_stats_with_meta}

In this section, we consider additional product meta fields to gain insights into what can be beneficial for better predictions of summaries. It is reasonable to assume that the summary writer had read additional information on the Amazon product page before he wrote the summary. Consequently, if a summarizer conditioned on such information, it can make better predictions.

We consider two main fields that are readily available in provided meta data, namely, \textit{features} and \textit{description}. Features and descriptions have average lengths of 101.3 ($\sigma=75.81$) and 182 ($\sigma=302.72$) words, respectively. Further, we calculate statistics as in Sec.~\ref{sec:summary_statistics} by also adding aspect precision (AP) as described in Appendix~\ref{app:aspect_based_metric}, and show results in Table~\ref{table:summary_stats_with_meta}. The results show an increase in text overlap when additional fields are added, which, in turn, suggests a potential for better predictions when the decoder has access to these fields. In our manual investigation, we found that often information present in \pc{} can be found in one of the fields. For example, different colors of the product are rarely mentioned in user reviews, however, it can often be found in the description.

\begin{table*}[h!]
    \centering 
    \begin{tabular}{l | c c c | c c c | c c c}
    \multicolumn{1}{c}{} & \multicolumn{3}{c}{\textbf{Verdict}} & \multicolumn{3}{c}{\textbf{Pros}} & \multicolumn{3}{c}{\textbf{Cons}}\\\thickhline
     & AP & R1 & R2 & AP & R1 & R2 & AP & R1 & R2\\
    \thickhline
    BR & 79.9 & 82.4 & 34.5 & 73.32 & 79.12 & 29.75 & 83.24 & 82.19 & 33.58 \\ 
    + feat & 82.0 & 84.0 & 36.0 & 78.95 & 83.12 & 33.88 & 84.28 & 82.85 & 34.05 \\
    + desc & 81.7 & 83.7 & 35.7 & 77.03 & 81.76 & 32.18 & 84.07 & 82.77 & 33.93 \\
    + both & 83.1 & 84.7 & 36.8 & 80.64 & 84.31 & 35.17 & 84.77 & 83.22 & 34.29 \\ 
    \thickhline
    CNET & 73.9 & 81.1 & 34.7 & 69.84 & 77.85 & 30.04 & 66.66 & 75.16 & 25.84 \\
    + feat & 75.1 & 81.7 & 35.3 & 72.29 & 79.73 & 31.47 & 68.10 & 76.08 & 26.24 \\
    + desc & 77.2 & 83.1 & 37.2 & 75.17 & 81.89 & 33.67 & 70.41 & 77.58 & 27.09 \\
    + both  & 77.6 & 83.4 & 37.5 & 76.27 & 82.61 & 34.39 & 71.08 & 77.98 & 27.34 \\ 
    \thickhline
    PM & 66.1 & 76.1 & 28.3 & 59.66 & 65.53 & 16.09 & 56.44 & 62.08 & 13.81\\
    + feat & 68.7 & 77.8 & 29.6 & 63.68 & 69.36 & 17.87 & 58.72 & 63.73 & 14.37\\
    + desc & 70.0 & 79.6 & 31.7 & 65.54 & 70.52 & 18.36 & 59.88 & 64.73 & 14.81 \\
    + both & 71.4 & 80.3 & 32.4 & 67.74 & 72.57 & 19.49 & 61.38 & 65.59 & 15.15 \\ 
    \thickhline
    RR & 42.3 & 60.5 & 13.1 & 42.46 & 59.44 & 13.47 & 46.90 & 63.11 & 16.02 \\
    + feat & 47.3 & 62.0 & 13.7 & 47.18 & 61.04 & 13.96 & 51.86 & 64.28 & 16.29 \\
    + desc & 48.6 & 63.6 & 15.1 & 47.71 & 62.17 & 15.04 & 51.52 & 65.10 & 17.32 \\
    + both & 51.8 & 64.6 & 15.5 & 50.96 & 63.21 & 15.35 & 55.01 & 65.83 & 17.48 \\ 
    \thickhline
    All & 76.9 & 81.0 & 33.2 & 70.90 & 77.40 & 28.31 & 78.82 & 79.69 & 31.10 \\
    + feat & 79.2 & 82.5 & 34.6 & 76.15 & 81.11 & 31.93 & 80.13 & 80.45 & 31.56 \\
    + desc & 79.2 & 82.5 & 34.6 & 74.94 & 80.29 & 30.79 & 80.19 & 80.59 & 31.61 \\
    + both & 80.6 & 83.5 & 35.6 & 78.25 & 82.59 & 33.38 & 81.06 & 81.07 & 31.95 \\ 
    \thickhline
    \end{tabular}
    \caption{Summary statistics of the dataset when additional meta data fields are added. ROUGE precision scores are used.}
    \label{table:summary_stats_with_meta}
\end{table*}
