# Supplementary material for: Learning Opinion Summarizers by Selecting Informative Reviews
Source: arXiv:2109.04325 source file (2021-09-09)
Supplement: Supplementary file 3 [file elbo.tex]

\subsection{ELBO}
\label{app:elbo}

We investigated whether the prior, regularizing the system is beneficial. As one could argue that the latent codes (reviews) being unable to produce one-to-one mapping to the summary are regularized by design, and thus no prior is needed.

We investigated different how \textsc{VSum} reacts to to different KLD scalars that are set during training.
