# Supplementary material for: Learning Opinion Summarizers by Selecting Informative Reviews
Source: arXiv:2109.04325 source file (2021-09-09)
Supplement: Supplementary file 4 [file posterior_collapse.tex]

\subsection{Posterior Collapse}
\label{app:posterior_collapse}

We observed that our variational model is able to recover from the early training phase posterior collapse without explicit annealing mechanisms. Posterior collapse has plagued text-related VAE models with strong decoders \citep{bowman2015generating, he2019lagging, pelsmaeker-aziz-2020-effective, brazinskas2020-unsupervised}. In such models, the decoder $p_{\theta}(x|z)$ ignores the latent code $z$ and rely solely on language model (local) statistics. Additionally, the approximate posterior $q(z|x)$ degenerates to the prior $p(z)$. While there are many explanations of the phenomenon, it's commonly believed that the learning dynamic is the central reason for the problem \citep{he2019lagging}. In the beginning of training, the model finds a local optimum in ignoring the latent code $z$ as it conveys no information about the datum $x$. After the collapse, it never manages to recover and the decoder $p_{\theta}(x|z)$ effectively is trained as the language model $p_{\theta}(x)$. 

The major difference in our approach is that latent codes are reviews, which are \textit{selected} as opposed to be \textit{learned} by the inference network. This implies that the approximate posterior always has to select $K$ reviews and their content can't be adjusted. Consequently, in the early stages, the system can ignore the reviews as the decoder is not yet well trained to use them. However, as later stages where local statistics are exhausted, the decoder starts utilizing the input reviews and the inference network is consequently able to find better subsets. 

\arthur{TODO: add an illustration here!}
