# Supplementary material for: Learning Opinion Summarizers by Selecting Informative Reviews
Source: arXiv:2109.04325 source file (2021-09-09)
Supplement: Supplementary file 5 [file posterior_selected_subsets.tex]

\subsection{Posterior-Selected Review Subsets}
\label{sec:posterior_selected_review_subsets}

% Review lengths, on average
We perform extra experiments to understand why \ours{} model performs better than \ROUGE{}. Recall, their difference is only in the review selector used in training. \ours{} learns a neural model to approximate the posterior, whereas \ROUGE{} relies on a ROUGE heuristic. We hypothesize that the approximate posterior exploits more expressive features (beyond ROUGE) to select reviews which are more relevant to the summary, helping \ours{} to learn a stronger model, less prone to hallucinations. In order to validate this, in Table~\ref{table:posterior_res} we show their results on test set but in the training regime, i.e. with reviews  selected while accessing the actual gold summary. As in training, \ROUGE{} uses the ROUGE heuristic, while \ours{} relies on the learned posterior. Naturally, both methods obtain stronger scores in this artificial set-up (Table~\ref{table:posterior_res} vs. Table~\ref{table:example_4}). What is more interesting is that \ours{} is considerably stronger than \ROUGE{}, suggesting that the \ours's selection component indeed chooses more relevant reviews. 

%We observed that the posterior yields reviews result in substantially better verdict and pros summaries in terms of ROUGE. 

%using a learned posterior selector in training for \ours{} and relying on a ROUGE heuristic in training by \ROUGE{}. To do this we evaluate them in the training regime, i.e. with reviews  selected while accessing the actual gold summary. Here, we used the posterior and $\textsc{R1 top-k}$ heuristic and their corresponding summarizers, and the results are shown in Table~\ref{table:posterior_res}.

%posterior for \ours{}
%Fist, we observed that when the prior is used to select reviews for different models, reviews of different lengths on average are preferred. 
%Specifically, 77.14 and 83.13 words for \ours{} and \ROUGE{} respectively, yet random subsets are of 51.44 words long. 
%We further evaluate summaries generated based on reviews selected while accessing the actual gold summary. Here, we used the posterior and $\textsc{R1 top-k}$ heuristic and their corresponding summarizers, and the results are shown in Table~\ref{table:posterior_res}. We observed that the posterior yields reviews result in substantially better verdict and pros summaries in terms of ROUGE. We believe that it is caused by the posterior being able to learn better review selection using a multitude of features. 

\begin{table}[h!]
    \centering
    \begin{tabular}{l | c c c}
    \multicolumn{1}{c}{} & \textbf{Verdict} & \textbf{Pros} & \textbf{Cons} \\\thickhline
    & RL & RL & RL \\
    \thickhline
    % \textsc{R1 top-k} & 18.52 & 19.84 & 12.96 \\
    \textsc{R1 top-k} & 19.38 & 21.09 & 13.26 \\
    % \hline
    % \textsc{SeSum} & 18.87 & 19.15 & 13.21 \\
    \textsc{SeSum} & 20.50 & 20.96 & 14.76 \\ 
    \thickhline
    \end{tabular}
    \caption{Test set ROUGE F1 scores contrasting to review selection guided by the gold summary.}
    \label{table:posterior_res}
    \NoGap
\end{table}
