# Supplementary material for: Learning Opinion Summarizers by Selecting Informative Reviews
Source: arXiv:2109.04325 source file (2021-09-09)
Supplement: Supplementary file 6 [file reinforce.tex]

\subsection{REINFORCE}
\label{app:reinforce}

In this section, we provide more details how REINFORCE was applied to optimize \textsc{VSum}.
