# Supplementary material for: Learning Opinion Summarizers by Selecting Informative Reviews
Source: arXiv:2109.04325 source file (2021-09-09)
Supplement: Supplementary file 7 [file sum_lengths.tex]

\subsection{Generated Summary Lengths}
\label{app:generated_summary_lengths}

When beam search with the size of 5 was applied to our models, we observed that without length constraints, the ones that re-sample reviews at each epoch, tend to generate summaries that are shorter. While gold summaries are on average 83.66 words long, \textsc{RandSel} and \ours{} tend to generate summaries that are on average 62.56 and 58.58 words long, respectively. On the other hand, \ROUGE{} yields summaries that are 74.09 words long, on average. To match \ROUGE{}, we restricted summaries to be minimum of 75 subwords(~44 words) for \textsc{RandSel} and \ours{}. We investigated if the systems underestimate the summary length on a particular summary type or a subdomain. However, we found that they underestimate on every summary type and subdomain. 

We hypothesize that re-sampling leads to more uncertainty in the input space, and serves as a regularization. This, in turn, reduces the decoder's confidence in the output space, which leads to generation of shorter summaries.
